# Supplementary material for: LIBERO-MOR: A Multimodal Robustness Benchmark Across the Vision-Language-Action Pipeline
Source: arXiv:2611.28867 source file (2026-11-21)
Supplement: Supplementary file 1 [file manifest_audit.tex]

\begin{tabular}{lr}\toprule Metric & Value \\ \midrule
manifest\_sha256 & 2b1caa800b6fd9fd6420fad15b0eef1a000919dd365327b8313ac53ba4ef2d89 \\
num\_tasks & 40 \\
num\_variants & 13200 \\
seed\_indices & 0,1,2,3,4 \\
\bottomrule\end{tabular}
