# Supplementary material for: LIBERO-MOR: A Multimodal Robustness Benchmark Across the Vision-Language-Action Pipeline
Source: arXiv:2611.28867 source file (2026-11-21)
Supplement: Supplementary file 2 [file results_by_suite.tex]

\begin{tabular}{llrr}\toprule Model & Suite & Perturbed SR & RR \\ \midrule
OpenVLA-OFT & libero\_10 & 50.39 & 52.49 \\
OpenVLA-OFT & libero\_goal & 22.94 & 26.07 \\
OpenVLA-OFT & libero\_object & 71.70 & 71.70 \\
OpenVLA-OFT & libero\_spatial & 49.52 & 57.58 \\
pi0.5 & libero\_10 & 54.12 & 56.38 \\
pi0.5 & libero\_goal & 47.58 & 50.61 \\
pi0.5 & libero\_object & 83.52 & 85.22 \\
pi0.5 & libero\_spatial & 65.52 & 65.52 \\
UniVLA & libero\_10 & 29.82 & 43.85 \\
UniVLA & libero\_goal & 31.73 & 37.77 \\
UniVLA & libero\_object & 60.61 & 65.88 \\
UniVLA & libero\_spatial & 36.58 & 50.80 \\
GR00T-N1.7-LIBERO & libero\_10 & 51.94 & 54.10 \\
GR00T-N1.7-LIBERO & libero\_goal & 41.97 & 44.65 \\
GR00T-N1.7-LIBERO & libero\_object & 81.82 & 85.23 \\
GR00T-N1.7-LIBERO & libero\_spatial & 53.79 & 57.22 \\
AVA-VLA & libero\_10 & 50.52 & 52.62 \\
AVA-VLA & libero\_goal & 19.85 & 22.56 \\
AVA-VLA & libero\_object & 75.03 & 75.03 \\
AVA-VLA & libero\_spatial & 53.30 & 55.52 \\
TBD-VLA & libero\_10 & 52.97 & 55.18 \\
TBD-VLA & libero\_goal & 49.15 & 53.43 \\
TBD-VLA & libero\_object & 80.30 & 80.30 \\
TBD-VLA & libero\_spatial & 55.58 & 59.12 \\
CogACT-Libero & libero\_10 & 53.36 & 56.77 \\
CogACT-Libero & libero\_goal & 45.33 & 51.52 \\
CogACT-Libero & libero\_object & 78.91 & 78.91 \\
CogACT-Libero & libero\_spatial & 55.73 & 59.28 \\
\bottomrule\end{tabular}
