# Supplementary material for: LIBERO-MOR: A Multimodal Robustness Benchmark Across the Vision-Language-Action Pipeline
Source: arXiv:2611.28867 source file (2026-11-21)
Supplement: Supplementary file 3 [file software_environment.tex]

\begin{tabular}{ll}\toprule Component & Recorded value \\ \midrule
Python & 3.10.19 \\
Platform & Linux-5.15.0-139-generic-x86\_64-with-glibc2.31 \\
CUDA\_VISIBLE\_DEVICES &  \\
torch & 2.8.0+cu128 \\
numpy & 1.24.3 \\
mujoco & 3.4.0 \\
robosuite & 1.4.1 \\
libero & 0.1.0 \\
transformers & 4.40.1 \\
diffusers & 0.30.3 \\
jax & : package not installed in build interpreter \\
opencv-python & 4.6.0.66 \\
Pillow & 12.1.0 \\
PyTorch CUDA build & 12.8 \\
\bottomrule\end{tabular}
